# Supplementary material for: A Longitudinal Study of Static Analysis Warning Evolution and the Effects of PMD on Software Quality in Apache Open Source Projects
Source: arXiv:1912.02179 source file (2020-08-27)
Supplement: Supplementary file 1 [file rules_appendix.tex]

Basic Rules & Major & Avoid Branching Statement As Last In Loop & 5.0 (2012-05-01) & \\
Basic Rules & Critical & Avoid Decimal Literals In Big Decimal Constructor & 3.4 (2005-11-30) & FindBugs (DMI\_BIGDECIMAL\_CONSTRUCTED\_FROM\_DOUBLE)\\
Basic Rules & Major & Avoid Multiple Unary Operators & 4.2 (2008-03-25) & \\
Basic Rules & Critical & Avoid Thread Group & 3.6 (2006-03-29) & \\
Basic Rules & Major & Avoid Using Hard Coded IP & 4.1 (2007-11-17) & \\
Basic Rules & Critical & Avoid Using Octal Values & 3.9 (2006-12-19) & \\
Basic Rules & Minor & Big Integer Instantiation & 3.9 (2006-12-19) & \\
Basic Rules & Minor & Boolean Instantiation & 1.2 (2003-07-30) & Checkstyle (ExplicitInitialization)FindBugs (DM\_BOOLEAN\_CTOR)\\
Basic Rules & Critical & Broken Null Check & 3.8 (2006-10-04) & \\
Basic Rules & Critical & Check Result Set & 4.1 (2007-11-17) & \\
Basic Rules & Critical & Check Skip Result & 5.0 (2012-05-01) & \\
Basic Rules & Critical & Class Cast Exception With To Array & 3.4 (2005-11-30) & \\
Basic Rules & Minor & Collapsible If Statements & 3.1 (2005-05-10) & \\
Basic Rules & Critical & Dont Call Thread Run & 4.3 (2011-11-04) & FindBugs (RU\_INVOKE\_RUN)\\
Basic Rules & Critical & Dont Use Float Type For Loop Indices & 4.3 (2011-11-04) & \\
Basic Rules & Critical & Double Checked Locking & 1.04 (2003-03-21) & \\
Basic Rules & Critical & Empty Catch Block & 0.1 (2002-06-25) & Checkstyle (EmptyCatchBlock)\\
Basic Rules & Minor & Empty Finally Block & 0.4 (2002-07-10) & \\
Basic Rules & Major & Empty If Stmt & 0.1 (2002-06-25) & \\
Basic Rules & Minor & Empty Statement Block & 5.0 (2012-05-01) & \\
Basic Rules & Minor & Empty Statement Not In Loop & 1.5 (2004-02-02) & \\
Basic Rules & Minor & Empty Static Initializer & 1.5 (2004-02-02) & \\
Basic Rules & Major & Empty Switch Statements & 1.0 (2002-11-04) & \\
Basic Rules & Major & Empty Synchronized Block & 1.3 (2003-10-23) & \\
Basic Rules & Major & Empty Try Block & 0.4 (2002-07-10) & \\
Basic Rules & Critical & Empty While Stmt & 0.2 (2002-06-27) & \\
Basic Rules & Minor & Extends Object & 5.0 (2012-05-01) & \\
Basic Rules & Minor & For Loop Should Be While Loop & 1.02 (2003-01-22) & \\
Basic Rules & Critical & Jumbled Incrementer & 1.0 (2002-11-04) & \\
Basic Rules & Critical & Misplaced Null Check & 3.5 (2006-01-25) & \\
Basic Rules & Critical & Override Both Equals And Hashcode & 0.4 (2002-07-10) & Checkstyle (EqualsHashCode)FindBugs (HE\_EQUALS\_NO\_HASHCODE,HE\_HASHCODE\_NO\_EQUALS)\\
Basic Rules & Critical & Return From Finally Block & 1.05 (2003-04-17) & \\
Basic Rules & Major & Unconditional If Statement & 1.5 (2004-02-02) & \\
Basic Rules & Minor & Unnecessary Conversion Temporary & 0.1 (2002-06-25) & \\
Basic Rules & Critical & Unused Null Check In Equals & 3.5 (2006-01-25) & \\
Basic Rules & Critical & Useless Operation On Immutable & 3.5 (2006-01-25) & \\
Basic Rules & Minor & Useless Overriding Method & 3.3 (2005-09-15) & \\
Brace Rules & Minor & For Loops Must Use Braces & 0.7 (2002-07-25) & Checkstyle (NeedBraces)\\
Brace Rules & Minor & If Else Stmts Must Use Braces & 0.2 (2002-06-27) & Checkstyle (NeedBraces)\\
Brace Rules & Minor & If Stmts Must Use Braces & 1.0 (2002-11-04) & Checkstyle (NeedBraces)\\
Brace Rules & Minor & While Loops Must Use Braces & 0.7 (2002-07-25) & Checkstyle (NeedBraces)\\
Clone Implementation Rules & Major & Clone Throws Clone Not Supported Exception & 1.9 (2004-07-14) & \\
Clone Implementation Rules & Critical & Proper Clone Implementation & 1.4 (2004-01-07) & Checkstyle (SuperClone)FindBugs (CN\_IDIOM\_SUPER\_CALL)\\
Controversial Rules & Minor & Assignment In Operand & 1.03 (2003-02-11) & Checkstyle (InnerAssignment)\\
Controversial Rules & Major & Avoid Accessibility Alteration & 4.1 (2007-11-17) & \\
Controversial Rules & Minor & Avoid Prefixing Method Parameters & 5.0 (2012-05-01) & \\
Controversial Rules & Major & Avoid Using Native Code & 4.1 (2007-11-17) & \\
Controversial Rules & Minor & Default Package & 3.4 (2005-11-30) & \\
Controversial Rules & Major & Do Not Call Garbage Collection Explicitly & 4.2 (2008-03-25) & \\
Controversial Rules & Major & Dont Import Sun & 1.5 (2004-02-02) & Checkstyle (IllegalImport)\\
Controversial Rules & Minor & One Declaration Per Line & 5.0 (2012-05-01) & \\
Controversial Rules & Major & Suspicious Octal Escape & 1.5 (2004-02-02) & \\
Controversial Rules & Minor & Unnecessary Constructor & 1.0 (2002-11-04) & \\
Design Rules & Minor & Abstract Class Without Abstract Method & 3.0 (2005-03-23) & \\
Design Rules & Minor & Abstract Class Without Any Method & 4.2 (2008-03-25) & \\
Design Rules & Critical & Assignment To Non Final Static & 2.2 (2005-01-31) & \\
Design Rules & Minor & Avoid Constants Interface & 3.5 (2006-01-25) & Checkstyle (InterfaceIsType)\\
Design Rules & Major & Avoid Instanceof Checks In Catch Clause & 3.0 (2005-03-23) & \\
Design Rules & Minor & Avoid Protected Field In Final Class & 2.1 (2004-12-15) & \\
Design Rules & Minor & Avoid Protected Method In Final Class Not Extending & 5.1 (2014-02-11) & FindBugs (DLS\_DEAD\_LOCAL\_STORE,DLS\_DEAD\_LOCAL\_STORE\_OF\_NULL)\\
Design Rules & Minor & Avoid Reassigning Parameters & 1.0 (2002-11-04) & Checkstyle (ParameterAssignment)\\
Design Rules & Minor & Avoid Synchronized At Method Level & 3.0 (2005-03-23) & \\
Design Rules & Critical & Bad Comparison & 1.8 (2004-05-19) & \\
Design Rules & Minor & Class With Only Private Constructors Should Be Final & 4.1 (2007-11-17) & Checkstyle (FinalClass)\\
Design Rules & Critical & Close Resource & 1.2.2 (2003-10-06) & FindBugs (ODR\_OPEN\_DATABASE\_RESOURCE,ODR\_OPEN\_DATABASE\_RESOURCE\_EXCEPTION\_PATH,OS\_OPEN\_STREAM,OS\_OPEN\_STREAM\_EXCEPTION\_PATH,OBL\_UNSATISFIED\_OBLIGATION,OBL\_UNSATISFIED\_OBLIGATION\_EXCEPTION\_EDGE)\\
Design Rules & Critical & Constructor Calls Overridable Method & 1.04 (2003-03-21) & \\
Design Rules & Minor & Default Label Not Last In Switch Stmt & 1.5 (2004-02-02) & Checkstyle (DefaultComesLast)\\
Design Rules & Major & Empty Method In Abstract Class Should Be Abstract & 4.1 (2007-11-17) & \\
Design Rules & Critical & Equals Null & 1.9 (2004-07-14) & FindBugs (EC\_NULL\_ARG)\\
Design Rules & Minor & Field Declarations Should Be At Start Of Class & 5.0 (2012-05-01) & \\
Design Rules & Minor & Final Field Could Be Static & 1.1 (2003-06-19) & \\
Design Rules & Major & Idempotent Operations & 2.0 (2004-10-19) & \\
Design Rules & Minor & Immutable Field & 2.0 (2004-10-19) & \\
Design Rules & Major & Instantiation To Get Class & 2.0 (2004-10-19) & \\
Design Rules & Minor & Logic Inversion & 5.0 (2012-05-01) & \\
Design Rules & Critical & Missing Break In Switch & 3.0 (2005-03-23) & FindBugs (SF\_SWITCH\_FALLTHROUGH)\\
Design Rules & Minor & Missing Static Method In Non Instantiatable Class & 3.0 (2005-03-23) & \\
Design Rules & Critical & Non Case Label In Switch Statement & 1.5 (2004-02-02) & \\
Design Rules & Critical & Non Static Initializer & 1.5 (2004-02-02) & \\
Design Rules & Critical & Non Thread Safe Singleton & 3.4 (2005-11-30) & \\
Design Rules & Major & Optimizable To Array Call & 1.8 (2004-05-19) & \\
Design Rules & Critical & Position Literals First In Case Insensitive Comparisons & 5.1 (2014-02-11) & \\
Design Rules & Critical & Position Literals First In Comparisons & 3.3 (2005-09-15) & Checkstyle (EqualsAvoidNull)\\
Design Rules & Major & Preserve Stack Trace & 3.7 (2006-06-01) & \\
Design Rules & Major & Return Empty Array Rather Than Null & 4.2 (2008-03-25) & FindBugs (PZLA\_PREFER\_ZERO\_LENGTH\_ARRAYS)\\
Design Rules & Minor & Simple Date Format Needs Locale & 2.0 (2004-10-19) & \\
Design Rules & Minor & Simplify Boolean Expressions & 1.05 (2003-04-17) & Checkstyle (SimplifyBooleanExpression)\\
Design Rules & Minor & Simplify Boolean Returns & 0.9 (2002-08-16) & Checkstyle (SimplifyBooleanReturn)\\
Design Rules & Minor & Simplify Conditional & 3.1 (2005-05-10) & \\
Design Rules & Major & Singular Field & 3.1 (2005-05-10) & \\
Design Rules & Major & Switch Stmts Should Have Default & 1.0 (2002-11-04) & Checkstyle (MissingSwitchDefault)FindBugs (SF\_SWITCH\_NO\_DEFAULT)\\
Design Rules & Minor & Too Few Branches For ASwitch Statement & 4.2 (2008-03-25) & \\
Design Rules & Minor & Uncommented Empty Constructor & 3.4 (2005-11-30) & \\
Design Rules & Minor & Uncommented Empty Method & 3.4 (2005-11-30) & \\
Design Rules & Minor & Unnecessary Local Before Return & 3.3 (2005-09-15) & \\
Design Rules & Critical & Unsynchronized Static Date Formatter & 3.6 (2006-03-29) & FindBugs (STCAL\_STATIC\_SIMPLE\_DATE\_FORMAT\_INSTANCE,STCAL\_STATIC\_SIMPLE\_DATE\_FORMAT\_INSTANCE)\\
Design Rules & Major & Use Collection Is Empty & 3.9 (2006-12-19) & \\
Design Rules & Critical & Use Locale With Case Conversions & 2.0 (2004-10-19) & \\
Design Rules & Critical & Use Notify All Instead Of Notify & 3.0 (2005-03-23) & FindBugs (NO\_NOTIFY\_NOT\_NOTIFYALL)\\
Design Rules & Minor & Use Varargs & 5.0 (2012-05-01) & \\
Finalizer Rules & Major & Avoid Calling Finalize & 3.0 (2005-03-23) & FindBugs (FI\_EXPLICIT\_INVOCATION)\\
Finalizer Rules & Minor & Empty Finalizer & 1.5 (2004-02-02) & FindBugs (FI\_EMPTY)\\
Finalizer Rules & Critical & Finalize Does Not Call Super Finalize & 1.5 (2004-02-02) & Checkstyle (SuperFinalize)FindBugs (FI\_MISSING\_SUPER\_CALL)\\
Finalizer Rules & Minor & Finalize Only Calls Super Finalize & 1.5 (2004-02-02) & \\
Finalizer Rules & Critical & Finalize Overloaded & 1.5 (2004-02-02) & \\
Finalizer Rules & Critical & Finalize Should Be Protected & 1.1 (2003-06-19) & FindBugs (FI\_PUBLIC\_SHOULD\_BE\_PROTECTED)\\
Import Statement Rules & Minor & Dont Import Java Lang & 0.5 (2002-07-15) & Checkstyle (RedundantImport)\\
Import Statement Rules & Minor & Duplicate Imports & 0.5 (2002-07-15) & Checkstyle (RedundantImport)\\
Import Statement Rules & Minor & Import From Same Package & 1.02 (2003-01-22) & Checkstyle (RedundantImport)\\
Import Statement Rules & Major & Too Many Static Imports & 4.1 (2007-11-17) & \\
Import Statement Rules & Minor & Unnecessary Fully Qualified Name & 5.0 (2012-05-01) & \\
J2EE Rules & Critical & Do Not Call System Exit & 4.1 (2007-11-17) & \\
J2EE Rules & Major & Local Home Naming Convention & 4.0 (2007-07-20) & \\
J2EE Rules & Major & Local Interface Session Naming Convention & 4.0 (2007-07-20) & \\
J2EE Rules & Major & MDBAnd Session Bean Naming Convention & 4.0 (2007-07-20) & \\
J2EE Rules & Major & Remote Interface Naming Convention & 4.0 (2007-07-20) & \\
J2EE Rules & Major & Remote Session Interface Naming Convention & 4.0 (2007-07-20) & \\
J2EE Rules & Critical & Static EJBField Should Be Final & 4.1 (2007-11-17) & \\
JUnit Rules & Minor & JUnit Assertions Should Include Message & 1.04 (2003-03-21) & \\
JUnit Rules & Critical & JUnit Spelling & 1.0 (2002-11-04) & \\
JUnit Rules & Critical & JUnit Static Suite & 1.0 (2002-11-04) & FindBugs (IJU\_BAD\_SUITE\_METHOD,IJU\_SUITE\_NOT\_STATIC)\\
JUnit Rules & Minor & JUnit Test Contains Too Many Asserts & 5.0 (2012-05-01) & \\
JUnit Rules & Major & JUnit Tests Should Include Assert & 2.0 (2004-10-19) & \\
JUnit Rules & Minor & Simplify Boolean Assertion & 3.6 (2006-03-29) & \\
JUnit Rules & Minor & Test Class Without Test Cases & 3.0 (2005-03-23) & FindBugs (IJU\_NO\_TESTS)\\
JUnit Rules & Minor & Unnecessary Boolean Assertion & 3.0 (2005-03-23) & \\
JUnit Rules & Major & Use Assert Equals Instead Of Assert True & 3.1 (2005-05-10) & \\
JUnit Rules & Minor & Use Assert Null Instead Of Assert True & 3.5 (2006-01-25) & \\
JUnit Rules & Minor & Use Assert Same Instead Of Assert True & 3.1 (2005-05-10) & \\
JUnit Rules & Minor & Use Assert True Instead Of Assert Equals & 5.0 (2012-05-01) & \\
Jakarta Commons Logging Rules & Major & Guard Debug Logging & 4.3 (2011-11-04) & \\
Jakarta Commons Logging Rules & Minor & Guard Log Statement & 5.1.0 (2014-02-11) & \\
Jakarta Commons Logging Rules & Minor & Proper Logger & 3.3 (2005-09-15) & \\
Jakarta Commons Logging Rules & Major & Use Correct Exception Logging & 3.2 (2005-06-21) & \\
Java Logging Rules & Major & Avoid Print Stack Trace & 3.2 (2005-06-21) & \\
Java Logging Rules & Minor & Guard Log Statement Java Util & 5.1.0 (2014-02-11) & \\
Java Logging Rules & Minor & Logger Is Not Static Final & 2.0 (2004-10-19) & \\
Java Logging Rules & Major & More Than One Logger & 2.0 (2004-10-19) & \\
Java Logging Rules & Major & System Println & 2.1 (2004-12-15) & \\
JavaBean Rules & Major & Missing Serial Version UID & 3.0 (2005-03-23) & FindBugs (SE\_NO\_SERIALVERSIONID)\\
Naming Rules & Minor & Avoid Dollar Signs & 1.5 (2004-02-02) & \\
Naming Rules & Minor & Avoid Field Name Matching Method Name & 3.0 (2005-03-23) & \\
Naming Rules & Minor & Avoid Field Name Matching Type Name & 3.0 (2005-03-23) & \\
Naming Rules & Minor & Boolean Get Method Name & 4.0 (2007-07-20) & \\
Naming Rules & Minor & Class Naming Conventions & 1.2 (2003-07-30) & Checkstyle (TypeName)FindBugs (NM\_CLASS\_NAMING\_CONVENTION)\\
Naming Rules & Minor & Generics Naming & 4.2.6 (2011-09-14) & Checkstyle (ClassTypeParameterName,InterfaceTypeParameterName,MethodTypeParameterName)\\
Naming Rules & Minor & Method Naming Conventions & 1.2 (2003-07-30) & Checkstyle (MethodName)FindBugs (NM\_METHOD\_NAMING\_CONVENTION)\\
Naming Rules & Minor & Method With Same Name As Enclosing Class & 1.5 (2004-02-02) & Checkstyle (MethodName)FindBugs (NM\_METHOD\_CONSTRUCTOR\_CONFUSION)\\
Naming Rules & Minor & No Package & 3.3 (2005-09-15) & Checkstyle (PackageDeclaration)\\
Naming Rules & Minor & Package Case & 3.3 (2005-09-15) & \\
Naming Rules & Minor & Short Class Name & 5.0 (2012-05-01) & \\
Naming Rules & Minor & Short Method Name & 0.3 (2002-07-03) & \\
Naming Rules & Minor & Suspicious Constant Field Name & 2.0 (2004-10-19) & \\
Naming Rules & Critical & Suspicious Equals Method Name & 2.0 (2004-10-19) & FindBugs (NM\_BAD\_EQUAL)\\
Naming Rules & Critical & Suspicious Hashcode Method Name & 1.5 (2004-02-02) & FindBugs (NM\_LCASE\_HASHCODE)\\
Naming Rules & Minor & Variable Naming Conventions & 1.2 (2003-07-30) & Checkstyle (StaticVariableName,ParameterName,ParameterName,ParameterName,ParameterName,ConstantName)FindBugs (NM\_FIELD\_NAMING\_CONVENTION)\\
Optimization Rules & Minor & Add Empty String & 4.0 (2007-07-20) & \\
Optimization Rules & Major & Avoid Array Loops & 3.5 (2006-01-25) & \\
Optimization Rules & Minor & Redundant Field Initializer & 5.0 (2012-05-01) & \\
Optimization Rules & Major & Unnecessary Wrapper Object Creation & 3.8 (2006-10-04) & \\
Optimization Rules & Minor & Use Array List Instead Of Vector & 3.0 (2005-03-23) & \\
Optimization Rules & Major & Use Arrays As List & 3.5 (2006-01-25) & \\
Optimization Rules & Major & Use String Buffer For String Appends & 3.1 (2005-05-10) & \\
Security Code Guideline Rules & Major & Array Is Stored Directly & 2.2 (2005-01-31) & \\
Security Code Guideline Rules & Major & Method Returns Internal Array & 2.2 (2005-01-31) & \\
Strict Exception Rules & Major & Avoid Catching Generic Exception & 4.2.6 (2011-09-14) & Checkstyle (IllegalCatch)FindBugs (REC\_CATCH\_EXCEPTION)\\
Strict Exception Rules & Critical & Avoid Catching NPE & 1.8 (2004-05-19) & \\
Strict Exception Rules & Major & Avoid Catching Throwable & 1.2 (2003-07-30) & Checkstyle (IllegalCatch)\\
Strict Exception Rules & Major & Avoid Losing Exception Information & 4.2.6 (2011-09-14) & \\
Strict Exception Rules & Minor & Avoid Rethrowing Exception & 3.8 (2006-10-04) & \\
Strict Exception Rules & Minor & Avoid Throwing New Instance Of Same Exception & 4.2.5 (2009-02-08) & \\
Strict Exception Rules & Critical & Avoid Throwing Null Pointer Exception & 1.8 (2004-05-19) & \\
Strict Exception Rules & Major & Avoid Throwing Raw Exception Types & 1.8 (2004-05-19) & Checkstyle (IllegalThrows)\\
Strict Exception Rules & Critical & Do Not Extend Java Lang Error & 4.0 (2007-07-20) & \\
Strict Exception Rules & Critical & Do Not Throw Exception In Finally & 4.2 (2008-03-25) & \\
Strict Exception Rules & Major & Exception As Flow Control & 1.8 (2004-05-19) & \\
String and StringBuffer Rules & Major & Avoid Duplicate Literals & 1.0 (2002-11-04) & FindBugs (HSC\_HUGE\_SHARED\_STRING\_CONSTANT)\\
String and StringBuffer Rules & Minor & Avoid String Buffer Field & 4.2 (2008-03-25) & \\
String and StringBuffer Rules & Minor & Consecutive Appends Should Reuse & 5.1 (2014-02-11) & \\
String and StringBuffer Rules & Minor & Consecutive Literal Appends & 3.5 (2006-01-25) & \\
String and StringBuffer Rules & Minor & Inefficient String Buffering & 3.4 (2005-11-30) & \\
String and StringBuffer Rules & Critical & String Buffer Instantiation With Char & 3.9 (2006-12-19) & \\
String and StringBuffer Rules & Minor & String Instantiation & 1.0 (2002-11-04) & \\
String and StringBuffer Rules & Minor & String To String & 1.0 (2002-11-04) & \\
String and StringBuffer Rules & Minor & Unnecessary Case Change & 3.3 (2005-09-15) & \\
String and StringBuffer Rules & Critical & Use Equals To Compare Strings & 4.1 (2007-11-17) & Checkstyle (StringLiteralEquality)FindBugs (ES\_COMPARING\_PARAMETER\_STRING\_WITH\_EQ,ES\_COMPARING\_PARAMETER\_STRING\_WITH\_EQ)\\
Type Resolution Rules & Major & Clone Method Must Implement Cloneable & 3.9 (2006-12-19) & FindBugs (CN\_IMPLEMENTS\_CLONE\_BUT\_NOT\_CLONEABLE)\\
Type Resolution Rules & Major & Loose Coupling & 3.9 (2006-12-19) & Checkstyle (IllegalType)\\
Type Resolution Rules & Major & Signature Declare Throws Exception & 4.0 (2007-07-20) & \\
Type Resolution Rules & Minor & Unused Imports & 4.0 (2007-07-20) & Checkstyle (UnusedImports)\\
Unnecessary and Unused Code Rules & Major & Unused Local Variable & 0.1 (2002-06-25) & Checkstyle (FinalLocalVariable)FindBugs (DLS\_DEAD\_LOCAL\_STORE,DLS\_DEAD\_LOCAL\_STORE\_OF\_NULL)\\
Unnecessary and Unused Code Rules & Major & Unused Private Field & 0.1 (2002-06-25) & FindBugs (UWF\_UNWRITTEN\_PUBLIC\_OR\_PROTECTED\_FIELD,UWF\_UNWRITTEN\_PUBLIC\_OR\_PROTECTED\_FIELD,UWF\_UNWRITTEN\_PUBLIC\_OR\_PROTECTED\_FIELD,UUF\_UNUSED\_FIELD,URF\_UNREAD\_FIELD,UWF\_UNWRITTEN\_FIELD)\\
Unnecessary and Unused Code Rules & Major & Unused Private Method & 0.7 (2002-07-25) & FindBugs (UPM\_UNCALLED\_PRIVATE\_METHOD)\\
